# Supplementary material for: Of Dice and Games: A Theory of Generalized Boosting
Source: arXiv:2412.08012 source file (2024-12-11)
Supplement: Supplementary file 1 [file appendix-multi.tex]

\newpage
\section{Generalized Multiclass Boosting}

\subsection{Scalar-loss multiclass boosting}\label{subsec:multi:scalar}

\td{Add generalized definitions for the learners and the random dice.}

Let $\X$ be any domain and let $\Y = [k]$ for some integer $k \ge 2$. As usual, we fix a ground-truth labeling $f : \X \to \Y$.
We consider a general scalar loss function given by
\begin{align}
    \cost: \Y^2 \to \RR_{\ge 0}   
\end{align}
such that $\cost(i,i) = 0$ for all $i \in \Y$, and whose range is determined by the maximum $\norm{\cost}_{\infty} = \max_{i,j \in \Y} \cost(i,j)$. For instance, the standard 0-1 loss is the special case where $\cost(i,j)=\ind{i \ne j}$. Similarly to the binary case, we measure the power of a learner by comparing it to some kind of ``minimal'' learner that makes predictions without looking at the specific point at hand. To this end we consider again the following two-player zero-sum game. The first player starts by choosing a distribution $\D$ over $\X$. The second player is told the marginal distribution of $\D$ over $\Y$, that we denote by $\bq$, and it chooses a predictor $h: \X \to \Y$, possibly randomized. However, the distribution of the predictor's output $h(x)$ must be independent of $x$ for every $x \in X$; this means that $h(x) \sim \bp$ for some distribution $\bp$ over $\Y$ independent of $x$. The second player then pays the expected loss given by $\bq$ and $\bp$, that is, $\cost(\bq,\bp) = \E_{i\sim \bq}\E_{j \sim \bp}\cost(i,j)$. The smallest $z \in \RR_{\ge 0}$ such that the second player can always ensure $\cost(\bq,\bp) \le z$ regardless of $\bq$ is the value of the game, that is:
\begin{align}
    \val(\cost) \coloneq \max_{\bq \in \Delta_\Y} \min_{\bp \in \Delta_\Y} \cost(\bq,\bp) \;.
\end{align}
It will be of particular interest to \emph{restrict} the distributions $\bq$ which the first player is allowed to choose. Formally, for every $J \subseteq \Y$ define the value of the game restricted to $J$ as:
\begin{align}
    \val_J(\cost) \coloneq \max_{\bq \in \Delta_J} \min_{\bp \in \Delta_\Y} \cost(\bq,\bp) \;.
\end{align}

The definition of margin $\gamma(\cost, z)$ of a $(\cost, z)$-learner remains unchanged.
We also define a stronger notion of margin based on the values of the dice games restricted to subsets of $\Y$.
\begin{definition}
    The \emph{strong margin} of a $(\cost, z)$-learner $\A$ is
    \[
        \gamma^*(\cost, z) = \min\bigl\{\val_J(\cost) - z : J \subseteq \Y, \val_J(\cost) > z\bigr\} \;,
    \]
    where the minimum over the empty set is $0$.
\end{definition}
Once again, we shall write $\gamma^*$ instead of $\gamma^*(\cost, z)$ when both $\cost$ and $z$ are clear from the context.

A list predictor is a function $\L: \X \to 2^{\Y}$. For a distribution $\D$ over $\X$ and a labeling $f$, the \emph{failure probability} of $\L$ under $\D$ is:
\begin{align}
    \err_\D(\L) \coloneq \Pr_{x \sim \D} [f(x) \notin \L(x)]
\end{align}
A list predictor is \emph{based on} a learner $\A$ if there exists a finite sequence of hypotheses $(h_t)_{t=1}^T$ such that (i) every $h_t$ is returned by $\A$ on some input, and (ii) for every $x \in \X$ the list $\L(x)$ is a function of $(h_t(x))_{t=1}^T$.

\begin{algorithm}[H]
\caption{Scalar-loss multiclass boosting} \label{algorithm:multiclass:scalar} \label{alg:multiclass_boost}
\begin{algorithmic}[1]
    \REQUIRE sample $S = (x_i,y_i)_{i=1}^m$; accuracy $\delta > 0$; $(\cost, z)$-learner $\A$; parameter $\sigma > 0$
    \vskip3pt
    \STATE let $T = \operatorname{ceil}\Bigl(\frac{8\norm{\cost}_{\infty}^2 \ln(m)}{\sigma^2}\Bigr)$, $\eta = \sqrt{\frac{2 \ln(m)}{\norm{\cost}_{\infty}^2 T}}$, and $m_0 = m_0\bigl(\frac{\sigma}{2}, \frac{\delta}{T}\bigr)$, where $m_0$ is the sample complexity of $\A$.
    \STATE initialize: $D_1(i) = 1$ for all $i \in [m]$.
    \FOR{$t = 1, \dots, T$}
    \STATE compute the distribution $\D_t = \frac{D_t}{\sum_i D_t(i)}$ over $S$
    \STATE draw a multiset $S_t$ of $m_0$ labeled examples i.i.d.\ from $\D_t$ and obtain $h_t = \A(S_t)$
    \STATE for every $i = 1, \dots, m$ let:
    \[
        D_{t+1}(i) = D_t(i) \cdot e^{\eta \cdot \cost(y_i, h_t(x_i))} \;.
    \]
    \ENDFOR
    \STATE define $F: \X \times \Y \to \RR_{\ge 0}$ such that $F(x,y) = \frac{1}{T}\sum_{t=1}^T \cost(y, h_t(x))$ for all $x \in \X, y \in \Y$.
    \RETURN $H: \X \to 2^\Y$ such that, for all $x \in \X$,
    \[
        H(x) = \bigl\{y \in \Y : F(x,y) \le z + \sigma\bigr\} \;.
    \]  
\end{algorithmic}
\end{algorithm}

\begin{theorem}\label{subsec:multiclass:scalar:main_thm}
    Let $\X$ be any domain, let $\Y = [k]$, and let $\F \subseteq \Y^{\X}$.
    Fix any $f \in \F$ and let $S = \{(x_1, y_1), \dots, (x_m, y_m)\}$ be any multiset of examples labeled by $f$.
    Finally, let $\A$ be a $(\cost, z)$-learner for $\F$ with margin $\gamma > 0$ and strong margin $\gamma^* > 0$.
    Given $S$, any $0 < \sigma \le \norm{\cost}_{\infty}$ and $\delta > 0$, and oracle access to~$\A$, \Cref{alg:multiclass_boost} outputs a list predictor $H: \X \to 2^{\Y}$ such that:
    \[
        \Pr\bigl(\forall i \in [m],\, y_i \in H(x_i)\bigr) \ge 1 - \delta \;.
    \]
    Moreover, depending on the value of $\sigma$, $H$ satisfies the following:
    \begin{itemize} \setlength{\itemsep}{0pt}
        \item if $\sigma < \gamma$, then $H$ is a $(k-1)$-list predictor, i.e., $\max_{x \in \X} |H(x)| \le k-1$;
        \item if $\sigma < \gamma^*$, then $H$ returns only lists in $\J = \{J \subseteq \Y : \val_J(\cost) \le z\}$.
    \end{itemize}
\end{theorem}
\begin{proof}
    The first part of this proof follows similar steps as the one of \Cref{subsec:binary:scalar:main_thm}.
    In particular, fix any $i \in [m]$ and observe that, again by the regret analysis of Hedge and by the definitions of $\eta$ and $T$, \Cref{algorithm:multiclass:scalar} guarantees
    \begin{equation}\label{eq:multiclass_hedge_bound}
        \frac{1}{T} \sum_{t=1}^T \cost(y_i, h_t(x_i)) \le \frac{\sigma}{2} + \frac{1}{T} \sum_{t=1}^T \E_{j \sim \D_t}\bigl[\cost(y_j, h_t(x_j))\bigr] \;.
    \end{equation}
    Furthermore, since $\A$ is a $(\cost, z)$-learner for $\F$ and given the choice $h_t = \A(S_t)$, by a union bound over $t \in [T]$ we obtain that
    \begin{equation}\label{eq:multiclass_avg_loss_bound}
        \frac{1}{T} \sum_{t=1}^T \E_{j \sim \D_t}\bigl[\cost(y_j, h_t(x_j))\bigr] \le z + \frac{\sigma}{2}
    \end{equation}
    with probability at least $1 - \delta$.
    
    Now, we show that the list predictor $H$ built by \Cref{alg:multiclass_boost} satisfies $\err_\D(H) \le \epsilon$ with probability $1-\delta$.
    Precisely, by conditioning on the event given by the inequality in \Cref{eq:multiclass_avg_loss_bound}, we now demonstrate that $y_i \in H(x_i)$ for every $i \in [m]$.
    Consider the function $F: \X \times \Y \to \RR_{\ge 0}$ as defined by \Cref{alg:multiclass_boost}.
    Then, by \Cref{eq:multiclass_hedge_bound,eq:multiclass_avg_loss_bound} we obtain for every $i \in [m]$ that
    \begin{equation}
        F(x_i, y_i) = \frac{1}{T} \sum_{t=1}^T \cost(y_i, h_t(x_i)) \le z + \sigma \;,
    \end{equation}
    which in turn implies that $y_i \in H(x_i)$ by construction of $H$.
    
    We now proceed with characterizing the lists returned by $H$.
    Fix any $x \in \X$.
    Let $\bp^x \in \Delta_\Y$ be such that $p^x_y = \frac{1}{T} \sum_{t=1}^T \ind{h_t(x) = y}$ for any $y \in \Y$, and observe that $F(x,y) = \cost(y, \bp^x)$.
    
    First, assume that $\sigma < \gamma$.
    We can immediately observe that
    \begin{equation}
        \max_{y \in \Y} F(x,y)
        = \max_{y \in \Y} \cost(y, \bp^x)
        = \max_{\bq \in \Delta_\Y} \cost(\bq, \bp^x)
        \ge \max_{\bq \in \Delta_\Y} \min_{\bp \in \Delta_\Y} \cost(\bq, \bp)
        = \val(\cost) \;,
    \end{equation}
    meaning that there exists a label $\widetilde y \in \Y$ satisfying $F(x,\widetilde y) \ge \val(\cost)$, whereas the list $H(x)$ satisfies
    \begin{equation}
        \max_{y \in H(x)} F(x,y) \le z + \sigma = \val(\cost) - \gamma + \sigma < \val(\cost)
    \end{equation}
    by the properties of $\A$ and the definition of $\gamma > 0$.
    Hence, we infer that $\widetilde y \notin H(x)$ and thus $|H(x)| \le k-1$.

    Second, assume that $\sigma < \gamma^*$.
    Similarly to the previous chain of inequalities, we can show that the list $H(x)$ guarantees
    \begin{equation}
        \max_{y \in H(x)} F(x,y)
        = \max_{\bq \in \Delta_{H(x)}} \cost(\bq, \bp^x)
        \ge \max_{\bq \in \Delta_{H(x)}} \min_{\bp \in \Delta_\Y} \cost(\bq, \bp)
        = \val_{H(x)}(\cost) \;.
    \end{equation}
    Assume by contradiction that $H(x) \notin \J$, which then implies by definition of $\gamma^* > 0$ that
    \begin{equation}
        \gamma^* = \min_{J \notin \J} \val_J(\cost) - z \le \val_{H(x)}(\cost) - z \;.
    \end{equation}
    Then, by construction of $H$ we have that
    \begin{equation}
        z + \gamma^* \le \val_{H(x)}(\cost) \le \max_{y \in H(x)} F(x,y) \le z + \sigma < z + \gamma^* \;,
    \end{equation}
    which is a contradiction. Therefore, $H(x) \in \J$.
\end{proof}

\td{Generalization.}

\subsubsection{A lower bound for list learning}

The next result says that, if a learner $\A$ cannot ensure loss smaller than $\val_J(\cost)$ for some subset of labels $J$, then in general any list predictor based on $\A$ that is often correct must often output some superset of $J$.

\begin{theorem}
Let $\X$ be any domain, let $f : \X \to \Y$ be surjective, and let $\cost: \Y^2 \to \RR_{\ge 0}$ with $\cost(i,i)=0$ for all $i \in \Y$.
Fix $J \subseteq \Y$ nonempty and let $z \ge \val_J(\cost)$.
Then there exist a $(\cost,z)$-learner $\A$ and a distribution $\D^*$ over $\X$ such that every list predictor $\L$ based on $\A$ satisfies:
\[
    \Pr_{x \sim \D^*}[J \subseteq  \L(x)] \ge 1 - |J|\cdot\err_{\D^*}(\L) \;.
\]
\end{theorem}
\begin{proof}
Let $\X_J = \{x \in \X : f(x) \in J\}$ for any $J \subseteq \Y$.
Consider a learner $\A$ that, regardless of the input, returns the hypothesis $h: \X \to \Y$ defined as follows:
\begin{align}
    h(x) = \left\{
    \begin{array}{cc}
        f(x) & x \notin \X_J \\
        y \sim \bp^* & x \in \X_J
    \end{array}
    \right.
\end{align}
where $\bp^* \in \Delta_\Y$ is the distribution achieving $\val_J(\cost)$,
\begin{align}
    \bp^* \coloneq \arg \min_{\bp \in \Delta_\Y} \max_{\bq \in \Delta_J} \cost(\bq,\bp)
\end{align}
We first claim that $\A$ is a $(\cost,z)$-learner. To this end fix any distribution $\D$ over $\X$. Clearly if $\D(\X_J)=0$ then $L_\D(h)=0 \le z$; thus we may assume $\D(\X_J)>0$. Since $h(x)=f(x)$ for $x \notin \X_J$, and since $\cost(i,i)=0$ for all $i \in \Y$, then:
\begin{align}
    L_\D(h) &= \sum_{i,j \in \Y} \Pr_{x \sim \D}[f(x)=i \wedge h(x)=j]\cdot \cost(i,j)
    \\
    &= \sum_{i \in J}\sum_{j\in \Y} \Pr_{x \sim \D}[f(x)=i \wedge h(x)=j]\cdot \cost(i,j)
    \\
    &\le \sum_{i \in J}\sum_{j\in \Y} \Pr_{x \sim \D}[f(x)=i \wedge h(x)=j \,|\, x \in \X_J]\cdot \cost(i,j)
\end{align}
As $f(x)$ and $h(x)$ are independent for every $x \in \X_J$, and since $h(x) \sim \bp^*$ by definition of $h$, the last expression yields:
\begin{align}
    L_\D(h) &\le \sum_{i \in J}\sum_{j\in \Y} \Pr_{x \sim \D}[f(x)=i] \cdot p^*_j \cdot \cost(i,j)
\end{align}
The right-hand side equals $\cost(\bq,\bp^*)$ where $\bq \in \Delta_J$ is the marginal of $\D$ conditional on $\X_J$. We can then conclude by observing:
\begin{align}
    \cost(\bq,\bp^*) \le \max_{\bq \in \Delta_J} \cost(\bq,\bp^*) = \val_J(\cost) \le z
\end{align}
This proves that $\A$ is a $(\cost,z)$-learner.

Now let $\L: \X \to 2^{\Y}$ be a list predictor based on $\A$. Note that the distribution of $\L(x)$ is independent of $x$ for every $x \in \X_J$, and in particular is identical for all such $x$. Fix any set $U=\{x_1,\ldots,x_{|J|}\} \subseteq \X_J$ such that $f(x_j)=j$ for all $x_j \in U$, and let $\D^*$ be the uniform distribution over $U$.
Then:
\begin{align}
    \err_{\D^*}(\L) &= \Pr_{x \sim {\D^*}}[f(x) \notin \L(x)]
    \\ &= \Pr_{x \sim {\D^*}}[f(x) \in J \setminus \L(x)]
    \\ &= \E_{x \sim {\D^*}}\left[\frac{|J \setminus \L(x)|}{|J|}\right]
    \\ &= \frac{1}{|J|}\cdot\E_{x \sim {\D^*}}[|J \setminus \L(x)|]
    \\ &\ge \frac{1}{|J|}\cdot\Pr_{x \sim {\D^*}}[J \not\subseteq \L(x)]
\end{align}
Therefore:
\begin{align}
    1- \Pr_{x \sim {\D^*}}[J \subseteq \L(x)] = \Pr_{x \sim {\D^*}}[J \not\subseteq \L(x)] \le |J|\cdot\err_{\D^*}(\L)
\end{align}
We conclude that $\Pr_{x \sim {\D^*}}[J \subseteq  \L(x)] \ge 1 - |J|\cdot\err_{\D^*}(\L)$.
\end{proof}

\subsection{Vector-loss boosting}\label{subsec:multi:vector}

\subsection{Duality: scalar-loss $\leftrightarrow$  vector-loss}\label{subsec:multi:duality}
